# Supplementary material for: New curiosities in the menagerie of corks
Source: arXiv:2005.08928 ancillary file (2020-08-27)
Supplement: Supplementary file 1 [file README.pdf]

# Additional documentation for “New curiosities in the menagerie of corks”

KYLE HAYDEN  
LISA PICCIRILLO

This is a guide to the computer-assisted proofs in [3]. The calculations described rely on the software SnapPy [1], and these calculations can be verified by running SnapPy inside Sage [4]; the authors’ Sage activity logs are available at [2]. For additional information, see the official SnapPy documentation regarding verified computations.

## Calculations in the proof of Theorem 2

We follow the notation from the proof of [3, Theorem 2]. The claim to verify is that  $Y_0 \setminus \gamma$  admits a hyperbolic structure with isometry group isomorphic to  $\mathbb{Z}/2\mathbb{Z}$ . A surgery diagram for  $Y_0$  is depicted below, where the dashed curve represents  $\gamma$ .

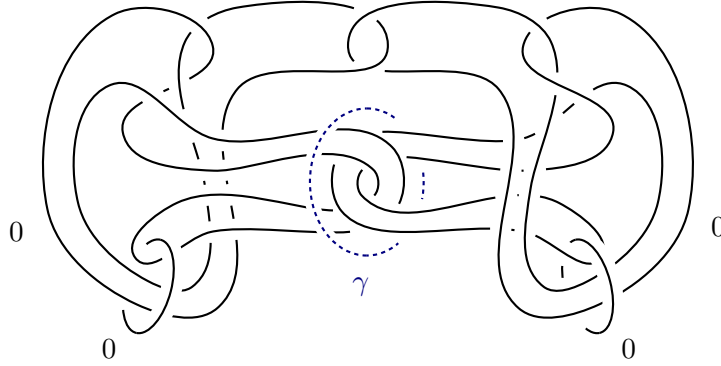

Figure 1

Together, the four surgery curves and  $\gamma$  form a five-component link  $L$  in  $S^3$ . We feed  $L$  to SnapPy using a planar diagram (PD) code. (This code was found via SnapPy’s link editor.)

```
In: L=Link([(26,82,27,81),(80,30,81,29),(65,1,66,42),(27,50,28,51),
(34,4,35,3),(7,21,8,20),(6,23,7,24),(5,33,6,32),(38,19,39,20),(39,25,40,24),
(4,11,5,12),(40,31,41,32),(41,13,42,12),(1,67,2,66),(51,28,52,29),
(17,82,18,83),(37,45,38,44),(2,36,3,35),(45,37,46,36),(47,22,48,23),
(46,9,47,10),(21,48,22,43),(79,14,80,15),(16,50,17,49),(52,16,53,15),
(77,65,78,64),(101,78,102,79),(98,84,99,83),(54,63,55,64),(89,63,90,62),
(84,61,85,62),(76,69,77,70),(55,71,56,70),(88,71,89,72),(85,73,86,72),
(58,68,59,67),(13,103,14,102),(100,54,101,53),(68,58,69,57),(93,73,94,74),
(94,61,95,60),(92,86,93,87),(8,43,9,44),(87,91,88,92),(74,96,75,91),
(59,96,60,95),(75,57,76,56),(25,97,26,104),(30,103,31,104),(18,97,19,98),
(99,90,100,49),(33,11,34,10)])
```

We then pass to the exterior of  $L$ :

```
In: A=L.exterior()
```

By default, SnapPy orders the link components so that  $\gamma$  is the last component, hence the last cusp (i.e. boundary component) of  $A = S^3 \setminus L$  corresponds to  $\gamma$ . We check that  $A$  admits a hyperbolic structure and then proceed to filling the first four cusps of  $A$ , producing  $Y_0 \setminus \gamma$ . (Inside Sage, one can verify hyperbolicity at each stage using the command `verify_hyperbolicity`, increasing the precision by setting the option `bits_prec` as needed.)

```
In: A.solution_type()
Out: 'all tetrahedra positively oriented'
In: A.dehn_fill((0,1),0)
In: A.solution_type()
Out: 'all tetrahedra positively oriented'
In: A.dehn_fill((0,1),1)
In: A.solution_type()
Out: 'all tetrahedra positively oriented'
In: A.dehn_fill((0,1),2)
In: A.solution_type()
Out: 'all tetrahedra positively oriented'
In: A.dehn_fill((0,1),3)
In: A.solution_type()
Out: 'all tetrahedra positively oriented'
```

Next we permanently fill the first four cusps so that SnapPy treats  $B = Y_0 \setminus \gamma$  as a hyperbolic 3-manifold with a single cusp, then we check for the hyperbolic structure on  $B$  and calculate its isometry group.

```
In: B=A.filled_triangulation()
In: B.solution_type()
Out: 'all tetrahedra positively oriented'
In: B.symmetry_group()
Out: Z/2
```

Inside Sage, we again need to use `verify_hyperbolicity`. Moreover, to rigorously compute the isometry group, we ask for a canonical retriangulation of  $B$  and then compute the isometry group of  $B$  via the isomorphisms of the canonical retriangulation:

```
In: K=B.canonical_retriangulation(verified = True)
In: len(K.isomorphisms_to(K))
Out: 2
```

### Calculations in the proof of Theorem 3

Following the notation from the proof of [3, Theorem 3], the claim to verify is that  $Y_0 \setminus \ell$  admits a hyperbolic structure with isometry group isomorphic to  $\mathbb{Z}/2\mathbb{Z}$ . Consider the link  $L \subset S^3$  shown in Figure 2, and note that  $Y_0$  is obtained by performing zero-framed Dehn surgery along all components  $L_1, \dots, L_7$  of  $L$ . Since  $\ell \subset Y_0$  corresponds to the meridians of the components  $L_6$  and  $L_7$  in the link  $L$ , the 3-manifold  $Y_0 \setminus \ell$  can be constructed alternatively from the exterior of  $L \subset S^3$  by performing zero-framed Dehn filling only along the components  $L_1, \dots, L_5$  of  $L$ .

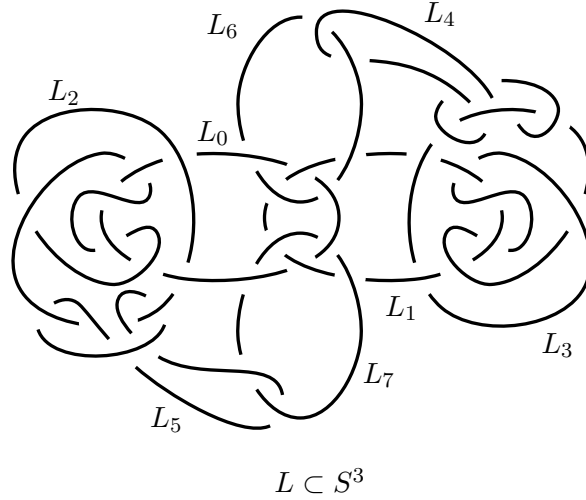

Figure 2

```
In: L=Link([(9,14,10,15),(6,18,7,17),(25,4,26,5),(11,36,12,25),(31,1,32,12),
(1,33,2,32),(33,3,34,2),(3,35,4,34),(35,31,36,30),(24,48,13,37),
(37,19,38,20),(39,24,40,23),(22,41,23,40),(41,22,42,21),(20,43,21,42),
(43,38,44,39),(51,47,52,46),(47,53,48,52),(53,51,54,50),(44,55,45,56),
(56,45,57,46),(54,57,55,58),(27,62,28,61),(62,27,63,26),(60,63,61,64),
(65,29,66,30),(28,66,29,67),(67,65,68,64),(15,74,16,69),(69,8,70,9),
(13,71,14,70),(49,71,50,72),(73,11,74,10),(72,58,73,49),(16,75,17,80),
(75,5,76,6),(76,60,77,59),(18,78,19,79),(68,78,59,77),(79,8,80,7)])
```

We then pass to the exterior of  $L$ :

```
In: A=L.exterior()
```

By default, SnapPy orders the link components of  $L$  using the same labeling as in Figure 2. We proceed to filling the first six cusps of  $A$ , producing  $Y_0 \setminus \ell$ . (It is not to verify hyperbolicity in Sage at this stage; that will come later.)

```

In: A.dehn_fill((0,1),0)
In: A.dehn_fill((0,1),1)
In: A.dehn_fill((0,1),2)
In: A.dehn_fill((0,1),3)
In: A.dehn_fill((0,1),4)
In: A.dehn_fill((0,1),5)

```

Next we permanently fill the first six cusps so that SnapPy treats  $B = Y_0 \setminus \ell$  as a hyperbolic 3-manifold with two cusps.

```

In: B=A.filled_triangulation()

```

Inside Sage, we ask for a canonical retriangulation of  $B$ , verify hyperbolicity, and then compute the isometry group of  $B$  via the isomorphisms of the canonical retriangulation:

```

In: K=B.canonical_retriangulation(verified = True)
In: K.solution_type()
Out: 'all tetrahedra positively oriented'
In: K.verify_hyperbolicity(bits_prec = 300)
Out: (True,
      [0.1148951498983...])
In: len(K.isomorphisms_to(K))
Out: 2
In: G=K.symmetry_group()
In: G.is_amphicheiral()
Out: True

```

It follows that the isometry group of  $Y_0 \setminus \ell$  has two elements, hence is isomorphic to  $\mathbb{Z}/2\mathbb{Z}$ . Indeed, Sage verifies that the nontrivial element is orientation-reversing, as described in [3].

## References

- [1] M Culler, N M Dunfield, M Goerner, J R Weeks, *SnapPy, a computer program for studying the geometry and topology of 3-manifolds*, <http://snappy.computop.org>
- [2] K Hayden, L Piccirillo, *Ancillary files for “New curiosities in the menagerie of corks”*, arXiv (August 2020)
- [3] K Hayden, L Piccirillo, *New curiosities in the menagerie of corks*, arXiv preprint (2020)
- [4] The Sage Developers, *SageMath, the Sage mathematics software system*, <https://www.sagemath.org> (2019)

Columbia University, New York, NY 10027

Brandeis University, Waltham, MA 02453

[hayden@math.columbia.edu](mailto:hayden@math.columbia.edu), [piccirli@mit.edu](mailto:piccirli@mit.edu)
