# Supplementary material for: New curiosities in the menagerie of corks
Source: arXiv:2005.08928 ancillary file (2020-08-27)
Supplement: Supplementary file 2 [file Sage_activity_log_Thm2.pdf]

In [1]: `import snappy`

In [2]: `L=snappy.Link([(26,82,27,81),(80,30,81,29),(65,1,66,42),(27,50,28,51),(34,4,35,3),(7,21,8,20),(6,23,7,24),(5,33,6,32),(38,19,39,20),(39,25,40,24),(4,11,5,12),(40,31,41,32),(41,13,42,12),(1,67,2,66),(51,28,52,29),(17,82,18,83),(37,45,38,44),(2,36,3,35),(45,37,46,36),(47,22,48,23),(46,9,47,10),(21,48,22,43),(79,14,80,15),(16,50,17,49),(52,16,53,15),(77,65,78,64),(101,78,102,79),(98,84,99,83),(54,63,55,64),(89,63,90,62),(84,61,85,62),(76,69,77,70),(55,71,56,70),(88,71,89,72),(85,73,86,72),(58,68,59,67),(13,103,14,102),(100,54,101,53),(68,58,69,57),(93,73,94,74),(94,61,95,60),(92,86,93,87),(8,43,9,44),(87,91,88,92),(74,96,75,91),(59,96,60,95),(75,57,76,56),(25,97,26,104),(30,103,31,104),(18,97,19,98),(99,90,100,49),(33,11,34,10)])`

In [13]: `A=L.exterior()`

In [14]: `A.cusp_info()`

Out[14]: `[Cusp 0 : complete torus cusp of shape -1.19084276226207 + 5.54799316443429*I,  
Cusp 1 : complete torus cusp of shape 0.216674882352546 + 3.09066319223597*I,  
Cusp 2 : complete torus cusp of shape -1.19084276226208 + 5.54799316443434*I,  
Cusp 3 : complete torus cusp of shape 0.216674882352547 + 3.09066319223596*I,  
Cusp 4 : complete torus cusp of shape 0.217460968026787 + 0.487807247077761*I]`

```
In [15]: A.verify_hyperbolicity(bits_prec=300)
```

3/26

4/26



```

72115198989317473937131276?*I,
  0.6546427065103505799793586741051281255477434833519613746466949478636332683
370490004882? + 1.53821683180035346024506538689143977864388706401014853491521
89204818516919001960557358?*I,
  0.4722375345647364223799668566338835438823620887963493020146707316702276374
552511037832? + 0.71949446011801741501945159270164287487876827205783122775412
27266588007291570329708459?*I,
  0.0167648415156838254270011730577804197907405337195651484763409161658575536
710491766233? + 0.73544796642041383152211743999229004401258401224448722947960
71575979393661602799431156?*I,
  0.6294536479519371342636844250870052152237454212303953262528236355126193444
600804099436? + 0.63930054818173369278274520790682133183163175478984188437866
37359703033927322534246717?*I,
  0.2876947483009901145052670997906993340834488609540602578364547222297844662
242317084850? + 0.38630126194268351044364767726837227118059112533644539462763
33846703618524132870029802?*I,
  0.5504034773220598604751008482016782558988130511870279191653586847359902583
124945508319? + 0.78113374685648443917649443673749120562444999834413738499722
32003737975733865449198023?*I,
  0.8168456271510927349753848972365844718279014333423313181593107394417925088
97677450156? + 1.017071257183962706932862240162225300111894805347854739279549
346541026882001135738573?*I,
  0.4584529259611814170976168864661995091441425086342557500219480662787277783
781247034014? + 0.49493254228394400635356432547777297067797439433489097369537
83932163882735753460368409?*I,
  0.3219524836272367118626594450630433246803298442896473246140640012553559736
987609965480? + 1.04690309470533265406799932635381753331533203608545241450854
91417008847134957274452614?*I,
  0.4210489383422082410228219889726033195658195703262080579960624016258683969
028116073490? + 0.86325756096532445910349628326910341164999989284513969871303
50512764986086617455625458?*I,
  0.3219524836272367118626594450630433246803298442896473246140640012553559736
987609965480? + 1.04690309470533265406799932635381753331533203608545241450854
91417008847134957274452614?*I,
  0.3281691544546958242353138031345910858530189546840743643496281575949886782
385263229213? + 0.74549926482466232769229782017852674075024306084100199314944
86775040861944179064254982?*I,
  1.1076625918552042949454300492722937484739306232685767010645231508582951276
63354740106? + 0.764816667643540298117789341725641564321973110654416602234089
9625256510611611515920198?*I,
  0.6065994057794761000165811990794586768835131958502990227307278229150623645
56377756125? + 0.876809080604284128770660420560407591708671186892647255478639
244471328750800203628279?*I])

```

In [16]: A.dehn\_fill((0,1),2)

```
In [17]: A.verify_hyperbolicity(bits_prec=300)
```

Out[17]: (True,  
[0.5658213859332661519586855708888685288341554342704571863905467374930908287  
958656390656? + 0.53849727313302753271442613165656363006854816624598992148526  
93947558578011844472706770? \* I,  
0.5658213859332661519586855708888685288341554342704571863905467374930908287  
958656390656? + 0.53849727313302753271442613165656363006854816624598992148526  
93947558578011844472706770? \* I,  
-0.153876645575087659323105265252232335869065009487717804194950829845210965  
9101614330404? + 1.0031971601581748629771193534969518170644235764213262992051  
161184590996276403237114169? \* I,  
0.5279210650990241908386889454309558074762212908632047376188721005034454392  
893311075200? + 0.79732547337536348988006244760776805183411073709515451508871  
63098262100418266783760891? \* I,  
0.5190978385260218928133659185118225624114268600196245800049152156669337424  
647451186753? + 0.60168034568366123561428795975914008389468317137250230962177  
00585231926229252075587133? \* I,  
0.6509463013321057051655297997617280122413756092237705283388182138070977932  
081937603055? + 0.48465905605959205570862438497002353325666611914129030406701  
40954579512116612314508333? \* I,  
0.4103876379280084349169827706439467453724595964449485967285424986098634724  
934492688112? + 0.50565567942963878164936098420080613248793737745250628497099  
60715691028528958760989949? \* I,  
0.4338682350992944733858420736853362784759008149353338478001730777974675726  
028148644527? + 0.59569197990023425164337272055937028727131642773228397549776  
67762440935740633920918205? \* I,  
-0.550574373793788160419737981070214226805161265286905844164631686285741354  
7823763541341? + 1.4893687624967737602761272054364889458695088255938972254018  
479852675088047854452400999? \* I,  
0.2884359184675155192920633501077752678980341450967217340089820170729443632  
130000844809? + 0.38430461369978734153764128836202185771341262431091838457964  
77379435502107121557180834? \* I,  
1.2691565813236677155558115775589943242977154374704908929019347714863834981  
518350072063? + 1.01175115470205261330196889717280004876096845510722323228334  
75983692495234978451484867? \* I,  
0.2419324005697324857864617192933008948195020657871472639509182636791492057  
287787616704? + 0.51773414655058592505328061364281634717184391278553227453452  
37396950757676278458591538? \* I,  
0.5507307375402692972114196639490258327072986248428973548202143801380739074  
520186155514? + 0.77940392186565592078996806010461858713269046144766021273286  
06277205864709761407189089? \* I,  
0.4605213813277026868342225142757390392841421641687520095632387806482900292  
731697833461? + 1.19775565216431076399106211484990550734474104689960695809401  
46109601980029786652435239? \* I,  
0.6306161079511190509877372991929488117913939734749399823165087239775330225  
521553301714? + 0.96990191162073103732727040785267874934029405320119803692916  
71442316114517792043333521? \* I,  
0.3841691016872146810842378183246746129477333709519139408402961784831694566  
2017662738885? + 0.4225445653066540591474524217381470659943190823534942232255  
2148279577802777914385270206? \* I,  
0.5449213333135667413995035153033736420303936814932205795588246005228970727  
842393296580? + 0.78289339789044357862728260055482694989216736252332189242628  
78675987871050647862101463? \* I,  
0.7774806756998195854591201745233795103666517896261057449638269640715586559  
538496091474? + 0.47736315707642960781969940796963791370187081148825435068173  
17740177767554918676023962? \* I,  
1.0659229788671979021448850507978313096585965564112213881241299417915826511  
269332632823? + 0.57351130349207306460828947099324612053937046076838477366180

66554665233398956053448344? \*I,  
0.4882832975312554773348055176556398289422278325501910199991390756200568135  
964342686132? + 0.77615612599382237345232130926205176191644519553517247428500  
95455002957799500918620760? \*I,  
-0.146039784104306230403597875130130976859472719388120710718331353320313860  
5844817929722? + 0.8765938539574221050102024897391039818502596112726393787438  
180036332732362961162631812? \*I,  
0.9763395309768883328350371139170559583497276749709942157805767749434209260  
95572809182? + 3.107420424756639086114400727591654712569943634940147695468416  
203390955270381242430793? \*I,  
0.9513013268768634330819162121295864207362533721971113676201736505971204543  
437181660313? + 0.45371789549434819421576797040655246707907810421014369335323  
68737638180220355579333866? \*I,  
0.4622864514400348409060047237600315961131608933050798721186597718127859901  
060191792564? + 0.97780118513017013038914311080890751239203423665293422648692  
95729153985142654953630020? \*I,  
0.8720250397166934229530385021708114876959067605247497161955921796248102831  
00707328220? + 1.318008742330946794933834271164901822950123629025707696827484  
7874160053756787673645003? \*I,  
0.0729815582316750687962591445342514696560788600954146279401532564608519001  
679261784715? + 0.75163400375620322887147520872462132531457449865717873559595  
16551981922978858658123028? \*I,  
0.2541136096891168147397204887506440004533921255658538578875858990158482050  
022669604680? + 0.54655590106410196078962682747059903376786764578725592443524  
01141414365899812123625721? \*I,  
0.3122940493307314385034725369641214736317160371129447789828599418807487469  
927016790045? + 0.67131417723486667152720181601674013203640813108470000971490  
95561890715078583791714001? \*I,  
0.5087165706226234849333781649115665761587866486210350788419087707423330454  
685899542973? + 1.11892479857964198842352328496574232703132743974447298404139  
91826911012040848061972044? \*I,  
0.5336789743445331763666507566328654209043426491230131439551623800367228413  
060750300351? + 1.34461050439052506408224623383618786562127654906051487495089  
28704899498368490609462275? \*I,  
0.7046849928132416832253675789332985348754276519997159697860063479327543197  
483568727443? + 0.38900033750504804764021937733800711172372270581723607290014  
03629462002622093634710988? \*I,  
0.5894446897241002613044385507942798684536833531287941776952945819254940590  
117596193557? + 0.79145908288510697002554794528213007600208998919541021804932  
08674339109460316067174370? \*I,  
1.1488216739916949816695030030896611498305440202020955414508893665046326789  
200547747691? + 0.71060918397568500245984627314194029481199359125148934569825  
03058787310458673617575496? \*I,  
0.7687592031206801042558127615886242098910917301775050686721757400581710307  
922167047878? + 1.36282322523468579008729148011873042675714951676281286906254  
9190752538265057742932440? \*I,  
0.5087165706226234849333781649115665761587866486210350788419087707423330454  
685899542973? + 1.11892479857964198842352328496574232703132743974447298404139  
91826911012040848061972044? \*I,  
1.5549613513996391709182403490467590207333035792522114899276539281431173119  
076992182947? + 0.95472631415285921563939881593927582740374162297650870136346  
35480355535109837352047923? \*I,  
0.0748316219609829820310656890444894298008452738688572058842824696294452681  
92089330853? + 2.462030510126245889969173101649478777298669348399481424462841  
445162237579026967044396? \*I,  
-0.244896057446156218347230603693404166539167557831705020769171562021123349  
4552507788036? + 1.5985745482174231125101977118985043211823589459674335729358

```

499124841785312883054781598?*I,
  1.8255786147667669689396701612833421671357537882066560248449579359509389682
64055822546? + 2.451786408373703658163780752503267535989833382900324644633545
710510748400796091699690?*I,
  0.8357923923726376410852010560467576282105423583764704673233093422293029123
825003711171? + 0.68037651717650538046567188318313094523684586854189070317311
17222079081740801178751253?*I,
  0.0337026473083456306729734761465991579365432772553430456647258776105204264
221086019798? + 0.60500190018988374579522464080820155430550818784710043675556
40011084649640759784722329?*I,
  0.6984373989353650303820159378050972512691893836088248992468244323510595208
960472952714? + 0.74846855453782575363020012066411359929650057183446347590020
78937927067319780517400911?*I,
  0.3744938217613698604424705048735776789229845050889314647646421761469773388
481629393523? + 0.35243424716251978835275837365670766599364694015652809725535
09331878892371181686757269?*I,
  0.2946074326313556698397366946095662805069896207122557116798848381886608280
761361568874? + 0.55952830749106117908271713209044048338262491256098968060915
93331371488901355089557607?*I,
  0.9078902134109544967889738930373282351777571660327194809857744329537601104
650639716094? + 0.61171806570802366100639070840267413376136576972096969596065
12032047071195985816085785?*I,
  0.5293149193277123087200780740922761493842485693617293993734369102115930898
291313878430? + 0.43532107173135143600116505541648454744813811440394168230095
20249217332904734759437138?*I,
  0.3538643388097282027048184122432120493039638739823494099171079055516308051
756392290333? + 1.12300622864485301041647627264938745075657748640212852332056
04573363214108462390050552?*I,
  0.7456589588376854983142140382916803932871833132945331734990107109104596502
19956972648? + 1.252211246231995690802201661056631766823636740293602928993604
369099525978510211671997?*I,
  0.1961080919384580546218844187760449610164628617882967345299402202643858868
067074331891? + 0.95730430910035894441739558068443604201956980836962445185460
81344305940914864290144429?*I,
  0.1416160161878392174885847726481063762065489656021329559175214342600676137
523631156175? + 1.29142262635439755068900029335026072456456271374986991010562
99387059848254385249054107?*I,
  0.9023357079846186900287075277855300407147631399854602145103333449933885441
64415833208? + 1.900835723069043371982074259417649318081868010807942545720180
519385948119733213181766?*I,
  0.6672454543474915751314424714272048349774078796269193035132761156170487970
03410358011? + 0.888031568465430684260473638811980300706611798290742617002180
3282597851437772180081418?*I])

```

In [18]: A.dehn\_fill((0,1),3)

```
In [19]: A.verify_hyperbolicity(bits_prec=300)
```

Out[19]: (True,  
[0.5829270000803952038688472331653533009797920651537035371132775686150793336  
877368782872? + 0.54525343145226696514488955749706099148369444905463749246743  
85285793231534910738407913? \* I,  
0.5829270000803952038688472331653533009797920651537035371132775686150793336  
877368782872? + 0.54525343145226696514488955749706099148369444905463749246743  
85285793231534910738407913? \* I,  
-0.118530152582348788191822174919744800840512555214722627905362738622572735  
0727357847667? + 1.0557454741221077946107407699264309040154683383802177225727  
526983711054834215458717386? \* I,  
0.5021658230568968207607895284194790195661583602800576581711106393823691444  
073651942928? + 0.80618297520014558974930078311406407118755112309168688801548  
19584316046010356277749348? \* I,  
0.5239246137994202387390274601461662957822648678895214752333059813329124932  
415984984707? + 0.61467460293541113059026272945752658006562472513608819741598  
25357822356716806885286370? \* I,  
0.6421435014466039887573082921163376299333587873693178420900603934351217905  
312131036989? + 0.47795663140898801050599831995293367891916205779956548132129  
03182724297917474193379161? \* I,  
0.4096873823609889665947066843378675592708860216210841153940140645497921764  
564985866941? + 0.51011407128911873728256380029023087258359005728502839558643  
44479787385837878705899246? \* I,  
0.4352077218005795228309866101084727223128505974765208634358245048079797350  
544016337663? + 0.60240774136271342134846891556496238268873590809208750139901  
03686257946879460837733167? \* I,  
-0.580375175162446641690662388787797733897564989148723310776505556906280607  
0098834079113? + 1.5102020052631934446722392273190852371847298193264323539613  
420236146848560209588624671? \* I,  
0.2870390296081661714979509343432806499575502834089324808873356583968732499  
808427132159? + 0.37746498990653495215710203320919230370410577900144973916520  
33558734495535424701189479? \* I,  
1.2686543295468242160211246094574615075906118445284350821204945888181199429  
300126504270? + 1.00540397277665252278723177600840755953159700573472722624233  
51287523758414573421014394? \* I,  
0.2367418978565408849167884256528538761038211943792359337064409456709436362  
619078953482? + 0.51635596247154157991563975529365892731992038633026433750109  
37314952814371790042475819? \* I,  
0.5486192752960283286812205515222485643956973868317557047532948589038790063  
055607411195? + 0.77402839864863912885305948431518799233954305444431585554447  
91693817015470023406266137? \* I,  
0.4595344274253768617865333853189737264431000489966909807601866873844432995  
955883301163? + 1.20829769966475596882152959613344603753155951230459223628470  
70777879521670570530226866? \* I,  
0.6332208174555241511107976817181221040205900282919551618017122071588280578  
939754878740? + 0.96859792607357964037211456555139093473138785124350927035850  
34476559748428842015658994? \* I,  
0.3721768412249216776388716117252854620984358410490058804754168922573065217  
113306146384? + 0.43160494887011927373362983610859960140779684008663050778178  
48623495901804252399142221? \* I,  
0.6089482513389243371221579006311194218316617707092514323843135627355900224  
781924855674? + 0.82036154353804637225607887723434679777056236803877218505009  
30163050100852461851785476? \* I,  
0.7367386293574269924455715794807495419767200751515889262493540252309407819  
505983772552? + 0.49663827884596180690780010155192389935011560081513816083867  
66543651240697829422961122? \* I,  
1.0667501013333667061810387043617240307126499250446141447247488559146960565  
521814902195? + 0.62910726401195003495711904260488617085911616839849042934924



71130348834701954468327565? \*I,  
0.4903057965969812381108275400667291687202354628700887060321958921273629112  
202383850497? + 0.77251767633932051635854621935204101440475716530148172662753  
82254583745618453767661088? \*I,  
-0.160035573734458453887760427782728807807967299271445868969267593943896429  
9648326159761? + 0.4053914697759582881544904946678009429969736798960618247745  
697128990496524781569236880? \*I,  
-0.802675051376675704356036992315471915364848885646904183996443964793268253  
859925386787? + 1.31519641889554202116530631925587629133235703238090892620288  
2626472575762003060786346? \*I,  
0.9930974117148256250847593247170146531735994463371563642003020463305105174  
907243022459? + 0.42074440949591563689880677183861043521679014375497997977645  
58891254531350369343137054? \*I,  
1.1898936811004850023684846110002147156863899674822986882721634516666165401  
806951190406? + 0.42403656600989067089341615489474832503454749706381719178648  
50145194081260088604285772? \*I,  
1.2467159164298466284518825940810077348730742816043898594791421919061436670  
544335568331? + 0.16613855596952140277902572301591472695041625376251720906514  
10595643042236419702447060? \*I,  
0.4438788847807933601090749162749997076781030065947057589176182191241184471  
574581925876? + 0.14329025040690160430894523250477091993126365040921663870709  
34401635950190106974426696? \*I,  
0.4766454857360105794722410241322598174702282844235257549497456985916537343  
716587296802? + 0.10985270704764242727756025204556954813482330704241617087998  
58323180172082133160993263? \*I,  
0.5513872687111617901520810633665720219039715794871621632429288083041905200  
886645230294? + 0.68043770928135045361054620885468146068987967391487064581753  
73739087069212388330514875? \*I,  
0.5097417287821077595541025669373122421881513767364340289552867031260904095  
224772441973? + 1.09999822621337279997560795463814794674832082104290310248536  
73007342827078741039364121? \*I,  
0.5267605274954776069640721403755602699969148555838298091768826194196653467  
198583976436? + 1.35300758253835467460590184442423897097732422141966399177668  
71643526026679536756827950? \*I,  
0.7078641489508812776641146366402150224199821545633223381524598959183125588  
425991620961? + 0.38705699052687583054135548306870362767857110753293520081293  
83208229727667105303828696? \*I,  
0.6095476320646220714658643406769105233982522357066239678338396970340384328  
975340014729? + 0.71182612986699175548250779151737544964800763689546186658257  
96477477472076797479900079? \*I,  
0.7320857183005583317607618750534290605206870592230660159018721227944631633  
703149611372? + 0.60729679567715270124015956454438552164147412906756525820383  
83954129621191468128112391? \*I,  
0.9840834495781332225326575278485444400292566959444008475031682663338838488  
759155220468? + 1.25672299264123513427966899737734836818057752028834318358184  
53754765608408110617410431? \*I,  
0.5097417287821077595541025669373122421881513767364340289552867031260904095  
224772441973? + 1.09999822621337279997560795463814794674832082104290310248536  
73007342827078741039364121? \*I,  
1.4734772587148539848911431589614990839534401503031778524987080504618815639  
011967545103? + 0.99327655769192361381560020310384779870023120163027632167735  
33087302481395658845922243? \*I,  
0.9540739563986491763630431430463881126629549189910099905913379188401664573  
87063593934? + 1.721769428493776154678443183235427754469572219439607552516682  
486811722037025972859141? \*I,  
-0.666297917556280263080414380195976612251589669557283525706632772057167565  
931796857381? + 2.52955549424212105890800540923146098127690330183174953741570



```

8673106290121544983426538?*I,
  1.3319295977726163100102947327405015608721397677959033081187960638610320795
00427831714? + 2.872439916494265013828881100685843971643905344272029196632451
518473288964601815453593?*I,
  0.7337094493615309736167671523672164541433828289502593930149621335531914673
815428185508? + 0.37998211407325443899122549878336862917935472735853617925718
66713432041362691545974977?*I,
  -0.095260919442036803369429958686635437671800306928418148517318778508850902
2823319127265? + 0.1359375379410299748498189361692210500358625813738854457983
065798461362722410387559425?*I,
  0.7312188716968860212500424210090297825832445219874725690151573829837403276
764547411901? + 0.65324882703153032683944847178222750800552793971030935089197
97239832250831695058881654?*I,
  0.0110586684627048619424142778261254728148451572781021732361643582600349062
693445508044? + 0.36275007820560693286826291678718807136250786524557382766316
65522930445560272478609301?*I,
  0.5366541464205138313240023086416534472929336496160434434683472783313475530
948984698199? + 0.70618634699207688700387646906101291518719138566498198332381
32546527691338440933200485?*I,
  0.7049438673928459522479379510627082647342770181689080569285503457376578390
642907556701? + 0.54094440422808668206391340798427087927129218750070044501525
65403044274376408133588896?*I,
  0.4899201643363234723871069791461982795197994912468287101000210410332990980
706757780855? + 0.30320703168223945998939098708486306028949183550720322796012
94991706244400124164039630?*I,
  0.1999912306172346299921304538007214821965864653080549620408501762072718057
06212777202? + 1.209605406702104462616004094269042227987261823071753401666663
7026456265718627476778791?*I,
  0.7209410180545311770179578346552582577302750046978927069778523025211530823
51784068725? + 1.347247038772239945092050320267449723711890477265482318888842
1462839965649781602090400?*I,
  0.0887255686247088090226197210108724978261093733991319314956307613332813641
050707586633? + 0.95951416762577971708244817377627561099372039693932545448982
08683200096899655770889507?*I,
  0.1677309620541875422006382603106047356465178702909778456749449612271148105
583914524971? + 0.96028393169759711476989982697677379681953964131493813096347
86854968548009885331314607?*I,
  0.2578183168480802102254509324272402670277243396401036488891459711057497299
23936303523? + 1.405052442575817807879934435881131797850372019733099270008952
008074412042501357472319?*I,
  0.5923361532365347736705576960447214146407655336874803460802615447995345697
47014018695? + 0.639870529691898388767345165332521959926766695071654487944233
3742395365712442865989231?*I])

```

In [20]: A.dehn\_fill((0,1),0)

```
In [21]: A.verify_hyperbolicity(bits_prec=300)
```

```
Out[21]: (True,
[0.6693376420180046221545162686612735789321127140376390275700954932269204149
559831850520? + 0.53454714796894581060619688565790557481283313778373120995187
68881091696657079616839722?*I,
0.6693376420180046221545162686612735789321127140376390275700954932269204149
559831850520? + 0.53454714796894581060619688565790557481283313778373120995187
68881091696657079616839722?*I,
-0.237639303997206803564658888674731214709938060236621722676082696097962874
8327832097321? + 0.8977212646861790670365635931150441650949739663992900923595
861752827947904247934576353?*I,
0.1298623373603770854241412925534310782315748710886149730313576371501165104
349154127503? + 0.75918289909619218668681308893189393603673228466233793081578
93287359130831248876282009?*I,
0.2400558009677663028572338282171037467748963216902357853309426730837023355
059244676277? + 0.53881881377894237857093390095944442504485532121095232828785
67845670924640547815059583?*I,
0.7321581809717248249239731207136170952164524116782103427415184396924983712
787469910663? + 0.45774005390931174063026710347175512672354724206397285892171
33646792395463790029005150?*I,
0.2776549211240733396183131474184150363281557525896702225275699502737382015
161207399636? + 0.69005787106182743112291523077755730100908658234906992820321
09488369768758628400950173?*I,
0.4680536365622883724475813812609745440633193285025179437443742570105464484
561667312957? + 0.97908551254163464414069533600853875141667717470084752299767
26674300039824546106700300?*I,
-0.318077344432455439923587753859460610560056824732178319907927607202618475
5041264843403? + 1.3664430579374610769692335170730581732221285608230846198500
978941883867246371187746222?*I,
0.3711076532355371996189771883414982063791639482903816625662896635383869280
600941704714? + 0.34577064174006021798394031412109771485344340606308404923561
41357132161268512599178847?*I,
1.4521159760774541928491979042104534189274939309579054005737691787836693485
447524213880? + 0.71780545483350338314660823805122855855926285147442980805388
82699656723573830278973604?*I,
0.0009477312546395150913083187432440372009219724796301410612390031481966494
9084103507237? + 0.3257887284115119301414000670264491103437718468638614666836
6846618383428149780432979808?*I,
0.2943316699991071082909889465290581039551489505280717253502123740423334013
045417196840? + 0.56238596462467979700277187552596758174299624667875571308440
59420024887213719413650065?*I,
0.3038649026857415206106692271817671520949151504782008361898718462873352819
926760455202? + 1.51569788448744019674482256300846652805009176154501000262300
42723076536580322188629399?*I,
1.1728525821486921015804162077711547923999582290306620335945293618295181738
010938386970? + 1.09566574719991820744640180517735180134944429842023572920745
50263460041401979110933703?*I,
0.7811518516613495339526739001073761321841286829487859462090010231184906670
5666530892207? + 0.4427507958790005484433459639244731126520549419240856817727
707964843218738811229354433?*I,
0.8016937647964191668477835071995487707462488830263351065514259227531031541
883129211973? + 0.47258875107215916090594943325852603154789686113096515408035
95890219321973541074019879?*I,
0.6871440087207541749371398381795431406419387582845481090146609233570197552
422406805235? + 0.27451607466580872658914038103781427591331534378083905643965
87679903709548512382853813?*I,
0.7450019653178298282004215008454345818809196415725471087595732123817819464
537509283542? + 0.50137544651758847967340609603708170831665766772600968042281
```

13058293780083799132280271? \*I,  
0.4529009235445867450247492658384468764285433665489947345041454299520338637  
717516994943? + 1.20464076069538287627297324256696756189152831685171186022208  
69197752222433010591567094? \*I,  
-0.158711345965626172513962573025160798805527668147828772677761762860207690  
4638130142352? + 0.4119052863249569410292349982112473742524993906903115734211  
627478373911788781268079816? \*I,  
-0.785559988440785589564572807282593606912452770629946524878987119885112803  
049791008321? + 1.30572853557725045236411006605555049427910537787549849825659  
72761258427599760303309855? \*I,  
0.9835098799565224317089248512339219424167816540839775828969421598079779786  
385626661634? + 0.42568650342191345931920393508322965948829102414279612674350  
58328328005533895812299017? \*I,  
1.1842233010042408927222957937115420545040289628260190895587461488050330172  
600602236664? + 0.42136555643899940368182255959101523172309587909117478235510  
84740221912892096243235806? \*I,  
1.2469872763692723299034221490429787739547045942803169413824756975502214278  
780085151135? + 0.16719102394436014419604779412798050806838253517526938932984  
91526249015609172151318572? \*I,  
0.4456490843261356482813832030058651204086220212829452817200169638346083536  
654071459568? + 0.14267274731057111027068240557201042231001745531745190557005  
29287966315610716911422674? \*I,  
0.4733297826639178581499241689466951965361228523512361018718493340560980632  
085639836055? + 0.11177431015466953959167719194876511645087457726070087247476  
70734829466119098437248334? \*I,  
0.5528108255842970991033677860849487475525450558323804031790936188311653055  
495093455958? + 0.68718718646483518721588789705831637572220568166143052027837  
47394500994987212563801580? \*I,  
0.3071547895671788207834566920918972494986587028760086795951526748213717972  
709525080541? + 2.10001427998101205327593449146248193378146439977472333586874  
21378569241020160910716232? \*I,  
0.6694647900193361413798626805757416855696320044358090925289749342321309894  
866782152305? + 0.59805670682340219316378086252200813613862124884509914574908  
83140711455541290763673846? \*I,  
0.6070860648544989352515011168724707265365770507174651785106855479881906291  
699680470367? + 0.23586464510220824816586765101973885152712604627356797624761  
77428700543889890450769466? \*I,  
0.6029539892310330179959207089687737755551834213938344873458525375341428801  
409950465772? + 0.65438013515782095930540355348730939560391119944833793505209  
52559327097389310672770751? \*I,  
0.7351622055119223470075431470247862096356754111293798171259483970889181147  
623918551659? + 0.60638725630024413939269940209551603009605064925642438443701  
73024049483940206357069895? \*I,  
0.7447196114062348956915443046910526692944844874801524596691168217490387351  
093630051537? + 1.29033493507688117507650560465163359242930518377052228970522  
03557490901759786033503104? \*I,  
0.9116218047333659231156974239212224746413064040235425524255708705764453494  
523387622967? + 0.74787278652708156396502472366924893699064218456909516621248  
76682120953980232596741612? \*I,  
1.7549763571163095190260312986551208163754371937409678815761045121384375467  
581010743186? + 1.79920380885816185931461168721528522648365671360189613483276  
5912770832351572666370607? \*I,  
0.9440612951637801002437583623198691559512146133332002051432915718662943002  
88764729432? + 1.681898444553577633840540850264246489769104961054176236269513  
838928644738209196605429? \*I,  
-0.658030127381220276345094420090886418414333589613065448467510114807333953  
919013125057? + 2.51623426315386307143015236387009024212579112053917946722462

```

3437615427868221169101221?*I,
  1.3170907971276966832081756599627773832545932823583448950158964659994594870
16597138239? + 2.824727105213187558017841890553479993327332560527206688012096
854332819356574400977897?*I,
  0.7288073296644917732033652619685386700338146836629918214767349742903541097
920536351387? + 0.37798517248319019188838362723802313241969304262068385920098
11838310578433114212084041?*I,
  -0.096188700278972530259446391053419446229381002890474197818590208517768703
1638290531397? + 0.1350210031480797905980466653463008857431725484489302249048
864843571455566674367312295?*I,
  0.7668301648706013228931774836164348392425874699787217312405160151806170584
350957962220? + 0.56387262527007236104692055744965176466629108316156009674392
91528919715077899803449694?*I,
  0.0095762206085856457196068138259210993252538992667069533430562653036568411
966175860437? + 0.36088857302428623592904242551431808342934299115893072352199
73206865335468300047917867?*I,
  0.5390063468375576267398139425728745984221135302206374969288729103453604435
560539556040? + 0.71566930094076528841994989604517386107762654437653185548468
16978747572164374932286400?*I,
  0.6940162282368897564519010216743141470218365632356358284072154163041404072
389907658752? + 0.54038869233773396092101134585053119274668002578429130308329
45325673308877034490274829?*I,
  0.5140120301575518025817655965987526326367621266059894705031590121815744464
879155487727? + 0.24936139872260827373853311504775677754017178210214374290153
09741615033715473918645803?*I,
  0.0635926334807211971956111746623812631675770171310091250990626918683183174
55801404936? + 1.066152239800479663786946195259647742307870827232020204658173
8262790819306042219077329?*I,
  0.7265593540131457571158357470279341051010926334734396950104853260067488792
959839609449? + 1.34695361576219965915550390621186756090603994896904729042311
58621404520693006669294101?*I,
  0.1066272672582349438978465498043685936970209387399192701719609609798073969
991524361733? + 1.02070143590787577841447765077998224308559987108951166057778
52485128688527862793022537?*I,
  0.1729786982279431807883356540558524113078923033147667980193149376641540914
779300276607? + 0.96276228698070645820887996917454012982949769103510372958209
85549283243794212380590308?*I,
  0.2919316212047119370809690919697801813503915231946600497973446030804272295
95904621591? + 1.387892075666876120777210725524405763713308754327109160089228
837831112344085819800763?*I,
  0.5201544915400400650207440767645037462732918424881235943864481949237783737
69546683287? + 0.727513331687585494577281622071675640816186191858753758475035
1611470388800774514193893?*I])

```

In [22]: A.dehn\_fill((0,1),1)

```
In [23]: A.verify_hyperbolicity(bits_prec=300)
```



Out[23]: (True,  
[0.2221239231118637340675083454325578660003690313671878616331724183053488204  
5210212973746? + 0.1095675136250992972526931118823367535975078218742195356456  
4498349937532832794033814488? \* I,  
1.7179289335779079810271029177144738560476827595693666038151764685476709473  
840344142567? + 0.41018472371057550489594005705765382808450773845858020389948  
03071219029750262335309224? \* I,  
-0.562376224059318616643111234201387470187471681964766511719796191158799240  
8651322541764? + 0.8318458119424232215616507541070308865299165608593636526419  
715290839397000066469452566? \* I,  
0.1152740129817744072445458161486627359430065378162568482827112381234675926  
216959106024? + 0.70338241229940519780830538390070112685296482963876452762848  
28529819194308331596831487? \* I,  
0.0932650099393102310865924199826754491942714315341501258613990492770741579  
088795278786? + 0.72006598876812070407425485157411173256343959082907813130413  
76216489231266652003423983? \* I,  
0.8951232655287948752742755775646862574657420807190353206876340128393899262  
0674188010080? + 0.1115386633490957691934237996323751463534791445774968600621  
8991242813750525567791014926? \* I,  
0.5794529249340391847168920201866107966308718531296008106197111142778600848  
544850502035? + 1.16505585777153334979415959576004616908299254979148407149769  
41447882382319205337623120? \* I,  
1.1843545697863750017480978645395964492714974737165624689037453188453405049  
265116147910? + 0.42813320748708669204582837059847064435233247385123079405215  
328432642824336798930636771? \* I,  
0.5892763922903163813816966090098847112358962425433880904972417643388005146  
781283954193? + 1.39422544107960074093466771765369039837887411849633467035031  
49352803035850621964400571? \* I,  
0.0165089332239716582965175272230289904893853309155348842853978848639071584  
756777560174? + 0.36310415166181869520264613722476103059510520291966617438878  
142634831159324778938889389? \* I,  
1.4748945930774762715673528052123580985069767360996864323928717367192519350  
5037185438892? + 0.2512516479848293907630379029751248327364142533198033979827  
5484405595823144663393706224? \* I,  
0.3570908454874613833643627866330003978870052865796979383326172752687801132  
1405713701439? + 0.2624649530392554785712845967204446618648917687692488104261  
6023982050265962234401596914? \* I,  
0.5308103982572067644495959207303808752349426522800110964137780412335357241  
630924145769? + 0.70809296470860552618520279051522111277520256374898772318528  
92940377398188646975402692? \* I,  
-1.029913818482174634520936038763683097238438357740442469357938268324500741  
5253794775035? + 0.4858252166948281485858787026972862112593143866637029433107  
627468282941634253522430137? \* I,  
1.8082592239098908450378229841357714954508802064078438974856514720348995768  
340550022006? + 2.07176630222487650765671276434436021556965589323332733421297  
22017926947621020984141372? \* I,  
0.8485139194667017478518559043671997779889250445328168983181769067584889228  
248880481226? + 0.71024257417421828926851476608601611061836878674830582364065  
72384288874572987268876753? \* I,  
0.7878491453872988125400567028906882695787818060703008155072636682350448889  
057232056126? + 0.52481488146892383217972713318567720854095292786484981210810  
64107471377818468984188942? \* I,  
0.6947456976792130941397374133367306076150610623126789392471590820162894297  
065159711954? + 0.30079827076891334965366620191477737600921074467254605076064  
67925688025930443753453825? \* I,  
0.7878491453872988125400567028906882695787818060703008155072636682350448889  
057232056126? + 0.52481488146892383217972713318567720854095292786484981210810

64107471377818468984188942?\*I,  
0.2941663263771872754665452015627601786207819700004194605635936996828043776  
393612313699? + 0.88631988596076993573122618870514000970099486384575874024249  
71008253665751815375042266?\*I,  
-0.163433314188662494146765897201875984461176206253775171672325821025372229  
2704353160478? + 0.4189196027470887609130231092853881455767611314511444159617  
415864092662116984528686808?\*I,  
-0.818165539054680543954317635073152668211266080867186257180530177571669803  
6940150688526? + 1.3363678706861040383940881405379369841302298680454523349796  
150515336758954067348490464?\*I,  
0.9748879687294611954352956390666937209291326826883904917024224001163950537  
113898954953? + 0.43419818829740890142470562681628517581555606829090938439481  
83815629273644399475546562?\*I,  
1.1843545697863750017480978645395964492714974737165624689037453188453405049  
265116147909? + 0.42813320748708669204582837059847064435233247385123079405215  
32843264282433679893063677?\*I,  
1.2605425827688576811421904631102111562813684486460110396052399304229888625  
600211979152? + 0.17755336706724103980383115975115200946460685811172484775757  
36120136299455608453495942?\*I,  
0.4492990283688769180761851284092549840771193593164092264136026151950015356  
877830724333? + 0.13148921441424319621277443823734168799538522902051052537710  
41768730760524546189124567?\*I,  
0.4659424514186682376889400656170389987894778821224580187530191187306430722  
450986282936? + 0.11151537093188261190102432144692493394165242452972624765917  
78786364554206645999179622?\*I,  
0.5498157062792352360722417807079011408019644692002069827786266676531485492  
673928458915? + 0.69040712040222769793303465744559543053322791637796121107238  
98703646910112376824701585?\*I,  
0.1327564305251516485188663544781313071615412000440019376302065289178658566  
818749365683? + 2.29541772220065003228352007713486867887038355385603025960772  
43153314180112399572909659?\*I,  
0.5098231128365244806425755909541302747043958962183424683239470007091416710  
3805287413759? + 0.6125301623064166674139696337649111316515387626837444120888  
795577354858167895122677529?\*I,  
0.6235285704650930065754774067555657516289182293216185423861185992945183486  
180486126841? + 0.32691931968547323358616835244823524887384816078052682163578  
60727769074587548332119418?\*I,  
0.4068072244206736614271581117890615227885829584161575375554890882718403249  
429665106562? + 0.80209797560744032076921246660159093107951288001376711003588  
04709946261002461809239721?\*I,  
0.7427988741073214055992701964175250144849505635151912452312721562814260491  
349399722715? + 0.60853677134450948570406446376753682491585342793010985080124  
69913021145427440315058887?\*I,  
0.8765349266165404411240256493727371523581680787975953698907614828846216292  
290054933297? + 1.41470583622009113378306507843459522124209297077130967533080  
63752945665159189512388363?\*I,  
0.8307727861991367562618373014760823296228053166646808628184311073264422389  
610876307000? + 0.98098584014061048192185098388759662450378913339113440364091  
98296537877345409856606735?\*I,  
1.6620638864046042945542625847311312194808418458036000722420715482678943684  
951263228700? + 1.63780146303254831222861862026142929513491057192290992309438  
62209629393421009939048010?\*I,  
0.9245993948171227568456815255373563378637287369521906986946105952066839241  
03417798287? + 1.667962498378478589810206133105425437995492352292784992219963  
446395550106065534081523?\*I,  
-0.654574534390254561619267540887445184740953152408260511955936091324767202  
8902708413701? + 2.5262549072586448744710156268086510726992834782936286671859



```

43464941142173170959392456?*I,
  1.3277948350071295806251327945938069630950445639014686125828808726625343698
112180280700? + 2.80978532362338553039355128466261699114871005653595944937405
18442436934920579895218603?*I,
  0.7290390802982131736261003747461507851286430520720568004181095463585677673
570456054703? + 0.38105762507277578750634712921410275613123441700283033367425
73826559299789469717482437?*I,
  -0.100083666402303046420910757430226935680241888446068801896709568953042324
1293929219738? + 0.1370781728594655846626916100939810822452723342968498486432
729896311126054289181271041?*I,
  0.6835278180772619761023223142192818669677511953265695735349612980965295745
777073692113? + 0.51077832630765977055774713396761315827937907484261078151711
21473881114610173455329439?*I,
  0.0165089332239716582965175272230289904893853309155348842853978848639071584
756777560174? + 0.36310415166181869520264613722476103059510520291966617438878
14263483115932477893888939?*I,
  0.5308103982572067644495959207303808752349426522800110964137780412335357241
630924145769? + 0.70809296470860552618520279051522111277520256374898772318528
92940377398188646975402691?*I,
  0.6763330826313445202988271077083125710077582555499191706777923785654025862
939268372385? + 0.53709678706557237358372733577695876114583644007519120133307
83534993342222599472166533?*I,
  0.4986858431837243195954462418314711161457929943293689420332522515522824696
569855349139? + 0.26551206024472072956923823178656001618586952976642285191641
57710854190919784354797809?*I,
  -0.069559801042273952421743402012468090864876681795559941923564885108641625
2797491497083? + 1.0612839719166102823805460455350350878951717139992968405299
967736141895754811708017325?*I,
  0.7730982470867503545619497892854164015077029082403154010380117506591955896
959063756529? + 1.38451588689220656609184865025087024906442940276271976956498
20693239741736087710919961?*I,
  -0.069559801042273952421743402012468090864876681795559941923564885108641625
2797491497083? + 1.0612839719166102823805460455350350878951717139992968405299
967736141895754811708017325?*I,
  0.1707690761003108395061193179417894255287680586736297979946289597707842336
195844431554? + 0.98992379432204969461668716530118854586999867644449935889464
19065261026813726541707049?*I,
  0.2872359146190397819078176457743362390956742435579715445452183247574574571
72056751212? + 1.346705747987649902963629407745813720102298254837756484167005
649140166471151620928686?*I,
  0.5960305776065210013719547818293001896134119896489046737660189850213611696
474512775344? + 0.80593516876773217070232451728252168728265604560602660697509
08632613872326155705326932?*I])

```

In [24]: B=A.filled\_triangulation()

```
In [25]: B.verify_hyperbolicity(bits_prec=300)
```

```
Out[25]: (True,
[-0.359120928191322992301485036832113736806481600328245816359838649730451330
0741503369? + 0.2480831457567848443861246312345557836943404257986598602913533
403929410960919881346? * I,
1.6019480591364398069556619287440729505440863321296231136385428355716219257
748819650? + 0.18477507743748186670010528328618989846586761039950554073887449
00957222515407665792? * I,
-0.617082291694544685749339334821641214608218420750609862990080382274882674
2832462840? + 1.4564364353522963773298693341272544138337166189507008362870874
247448897527600323739? * I,
0.8597380317069714454368136846659198187795156997842994179674463810042615583
235797487? + 0.68334135121148438376617254632114346979336600279696594001756446
47919283014321647108? * I,
0.4085468971435307324296536768933269790338912682968458071324717334194397477
696958083? + 0.54439501571251448777736127310436770988741506497880896614423482
70597301477097559371? * I,
0.0151221087168314075323105208098417848620791829845588469196586617071057792
406742452? + 0.70926768475297983100310544366989893602137017670863272395239121
72248348604200955059? * I,
1.0640949649973849346191158538521205126514010359695148243411091128851404055
475258950? + 0.37060637864496934555140916419808786700834208086306400127674997
77830396839092944945? * I,
0.0082635292348190279512432607364530982342214529815492854512409282770044571
796588191? + 0.73886286091213402139778694602235846249262427741431721971365002
21298735265914169844? * I,
-0.404509582614294166170685489634619548788547508372120954356385935479119922
4833916326? + 1.4084893396875608938423842189002111960123320692297985970278667
773802880400062800758? * I,
1.6328143983402049867944239939128794669587678332218091114827962881723493701
18044868? + 2.234245215303401240532038856938455370488199799441261900195643296
016659333873277641? * I,
-0.044330224488375615134394839493050215619340369089716419755554541743322933
1820202957? + 0.7242812169587339623001247227927297501187226317316039817326754
109871462986622036233? * I,
0.7795850906980381139155804736995911810948373177572622583964505564278967300
586345693? + 0.48604025868963334840243931576027207072327394390475486903077049
22042262882077065213? * I,
0.1652069292489004297771720061014351399404710547668875767376027001014183505
493450393? + 0.45546741857332726782942700024855930063835720101974695698724336
16810105990945518110? * I,
-0.423016357816415004829292996317063161765253535774308689940202296156882759
0533168099? + 0.1443941806113096640306599079833739072345276235146193474298711
207466061854433192311? * I,
0.3751732815113940232285703666721800477868792999111159642736737687640502303
122875509? + 0.47884309399385225714009712547463524876728454092739111851366826
90777892878943972431? * I,
0.5884896312761427165386808612730354209205350535057899009168381305934829766
731638268? + 1.52756038568174867399240427703105951821399539393277815154231248
33867948911234324570? * I,
0.4981481436622132511814343471640085098282481272296355577966701202081985350
209323255? + 1.30845631149673964285092566007806219974600307619487445896118166
76702629615774558088? * I,
-0.230745270172658924669244167734141772443209853406581661577066690855517098
0252552403? + 0.6657546317482075161637335150598630423195046587791860441065330
542177835558204047318? * I,
-0.020393485709973456387409169181910105670749752167361912932776011406974189
5669242474? + 0.708613927569822275592048405156953271589108881661669201303276
```

23400312211803784166? \*I,  
0.3460193545847318626598848558599238534154395282764655859055768149873812399  
586968121? + 0.73243776994207506391429152432900593120433720527594298817765264  
48858054928803389660? \*I,  
-0.074426713818239858548872654880367220948753296383448938629068443398729024  
2742305342? + 0.4093188523017931951717153149922175083732680586524774142914812  
959685885118670010431? \*I,  
0.7778269766210231880515152413006241645916137041935086130753945671501051709  
589844595? + 1.00835385579523416832360933196951875338344757916249827619207167  
60207979153620495633? \*I,  
1.5020465692196523330340748975592493278090289462474212340152568819162173264  
39476970? + 0.318805320644382516530463717906342312751825685478222166221555558  
548526199549319145? \*I,  
0.8437705117478947829597469900549776810186439530028539686785876581933208311  
57937040? + 1.527328856843840140114761316277769455451727326701329922364184086  
035416086987401428? \*I,  
1.2419406555675333267654487911617367402335806705075889815831226729922799864  
27842556? + 0.397979334127484953845148625827965109377379427289089868994845424  
4228607314549790976? \*I,  
-0.175411476376552383998777609376362761025419218535880062661842575592973283  
353709894? + 1.01673904451540075581537143923309353706868343817258201739915254  
7396265288093569073? \*I,  
0.7615512979596276493422913182151522332460903202417820700555831370127218653  
87530750? + 0.658693475576945821619773682132555277024644630223775233444416296  
5658681689602139427? \*I,  
0.8975310969414313917103345598429624953502506351208438022203594563052453904  
325208594? + 0.55079175354069437351261425098408297158234589076069250177737479  
80552969747247958019? \*I,  
0.8398388421338522634036188081471696184036584860088676232247975119349772012  
608493828? + 0.23769609842359885250238266702921963082788154317074502513797617  
38763715425442183920? \*I,  
0.2768270046539007204850331303818209702714144131570683903133068771158401265  
56804713? + 0.702242320260616785429151987635036214036451722793314109703855389  
3799841808750864745? \*I,  
0.7583161102633793409763459443677259627685658817248687357745749994524580387  
244420575? + 0.35369963438133191610677197872278630946075605582996150556108701  
00488798816775081382? \*I,  
0.2450112358500224174044941854521438025939583332506503652131663282886434006  
768686369? + 0.45383170647760756237412507396441417781193012961209451948718784  
06141077541754506379? \*I,  
-0.178153894146669426632981860104120050668333383846339637501646392755619625  
3982265338? + 0.0110861766778985601718536212807581297961869749393515527948622  
542222525897043526547? \*I,  
1.0676198273978725978770637051775103679151511216570483203485970794301246623  
094875006? + 0.91353780805610980268732053350819783405669999262212967103823706  
8438398654618449010? \*I,  
0.4173372275888896191997704129354635444408423420048537131692081853296567784  
68617311? + 2.69501849465758841968257799472502902390564519574144045050898540  
330614317775030153? \*I,  
0.8261280526964472678822351342742796377678208862437027439918537864010511266  
803029244? + 0.40910296713814486700559843458029449945888878582114597191684281  
73099615963441985784? \*I,  
0.3502837685949973571638612535469417730999271716962267067991467317778829788  
46194652? + 0.540278472654536159011534468346287126397343254127284733516910688  
018701031270969182? \*I,  
1.5846793178552769685564365827770146182685613710907733697000965844980079484  
07889453? + 1.043925069833247579638447957237906188263838208907618791221079338

```

132959035237334166?*I,
  0.2916743370218050529622457364309887542549575309624286555871542142296463601
83878290? + 1.627943918212566946115063093569747320368141904453246695868227983
979307038129595377?*I,
  0.2656752719129850792464091104024305540562107167874529089965106427376286564
086880107? + 0.49374437318599010223059118613650280128447496322013693559300174
40251206565272389805?*I,
  0.8327589979587951231898551911150252284180303040837718064093752400293706228
028445735? + 0.17476346666959164150758729223204560321985656282318174934291852
27193604794461389315?*I,
  1.0167245596334614021551353708090724971001270088856442253496622738757393559
098235769? + 0.19136895563181121179272977078264618692985028740950235600537727
91202779013292460627?*I,
  -2.620072274147449578517465158235031388148045960393290905565185669198108398
112603366? + 0.80325104714623225479645350434559635377821975090912386830563014
894319381379543793?*I,
  0.1114719675497612870107974570085334736284369944029184624634663296162381924
380221789? + 0.46212633730755292762862878142626553205021360506595864579895284
29535801994082919879?*I,
  4.5612494116264317856617592708066804681877204888691757963802474195976470023
2690307? + 7.1118267280608471446233117500605249552504063049127221528985907655
0831927107473729?*I,
  -0.267221675462245455369551529347939422328209381756450094169911321656046664
362937661? + 1.03479072459932855744524848411800654731761709166158570398185840
7766344668842092432?*I,
  0.9226193846782383867396996742709729216442115699728757547235370502535003356
611919306? + 0.62542053197478370733902322083984864862615758989280584886076314
57750703557207288512?*I,
  1.7648957297641069756968692946259705190556488448593663057922868176995727812
82000619? + 4.487239862140795903588551935020154476712431582266283093476118188
608341184438307736?*I,
  -4.283298294835845474959504457693643579212261338913540430942230195872107383
61394352? + 14.12183605939153707521672671626296277908138996945109964682217822
871543908408139997?*I,
  1.4634822045158599648186610084146910770095813545875015681929349078671823899
787761588? + 0.13228649639750068667498964076213033404878992857962529295867262
15755207332681966578?*I,
  0.3493312293240933702684103799182656844529977651957850699673314272496460908
864498839? + 0.67016082096501414734422116090501763832638655829859079308944492
06845380577017755280?*I,
  0.9926681368425664901097679045212931758357854499427630518564725196065767197
97249566? + 2.291734382302952217949231139416559208847537749690468461954699183
348011507338955158?*I,
  0.3125806947677741457882084167890756714062560538126243790509767374788400403
265536134? + 0.59103139557983469182739138469008475223583304222972260045177781
34985190477469526886?*I,
  0.9001593101774470897983958968320530070452444974944556374670362435983329674
270001037? + 0.46909852342888629264732639896067138442581944921988300811402632
80047889429522086970?*I])

```

In [26]: `K = B.canonical_retriangulation(verified = True)`

In [27]: `len(K.isomorphisms_to(K))`

Out[27]: 2

In [ ]:
