# Supplementary material for: New curiosities in the menagerie of corks
Source: arXiv:2005.08928 ancillary file (2020-08-27)
Supplement: Supplementary file 3 [file Sage_activity_log_Thm3.pdf]

# Verified computations for Theorem 3

August 25, 2020

```
In [1]: import snappy
```

Plink failed to import tkinter.

```
In [2]: L=snappy.Link([(9,14,10,15),(6,18,7,17),(25,4,26,5),(11,36,12,25),(31,1,32,12),
(1,33,2,32),(33,3,34,2),(3,35,4,34),(35,31,36,30),(24,48,13,37),(37,19,38,20),
(39,24,40,23),(22,41,23,40),(41,22,42,21),(20,43,21,42),(43,38,44,39),
(51,47,52,46),(47,53,48,52),(53,51,54,50),(44,55,45,56),(56,45,57,46),
(54,57,55,58),(27,62,28,61),(62,27,63,26),(60,63,61,64),(65,29,66,30),
(28,66,29,67),(67,65,68,64),(15,74,16,69),(69,8,70,9),(13,71,14,70),
(49,71,50,72),(73,11,74,10),(72,58,73,49),(16,75,17,80),(75,5,76,6),
(76,60,77,59),(18,78,19,79),(68,78,59,77),(79,8,80,7)])
```

```
In [3]: A=L.exterior()
```

```
In [4]: A.dehn_fill((0,1),0)
```

```
In [5]: A.dehn_fill((0,1),1)
```

```
In [6]: A.dehn_fill((0,1),2)
```

```
In [7]: A.dehn_fill((0,1),3)
```

```
In [8]: A.dehn_fill((0,1),4)
```

```
In [9]: A.dehn_fill((0,1),5)
```

```
In [10]: A.solution_type()
```

```
Out[10]: 'contains negatively oriented tetrahedra'
```

```
In [11]: B=A.filled_triangulation()
```

```
In [12]: B.solution_type()
```

```
Out[12]: 'contains negatively oriented tetrahedra'
```

```
In [13]: B.volume()
```

```
Out[13]: 50.7801274149449
```

```
In [15]: K=B.canonical_retriangulation(verified = True)
```

```
In [16]: K.solution_type()
```

```
Out[16]: 'all tetrahedra positively oriented'
```

```
In [17]: K.verify_hyperbolicity(bits_prec = 300)
```

```
Out[17]: (True,  
[0.11489514989830000443312263758511763399949873330219228153906041881486316296623889244  
-8.3314448865464576072681301263403891908158724991609068732210290563657350040610080837  
-0.2463382901665493722414387496123370420797260125744516744058196925365030691754092321  
-0.2032957106761212077513652827797140529021521914660693552227252291846608527652939814  
0.48978961928994195476959809701688528476429403755399658798243632193810318105932311054  
-0.5640086658743316949169649504841057627079507493269692657938970918611446816147705019  
0.31271105625817825711010599919985330248171739583324878127837185945905155586992338452  
1.8389311593679992422571918238755946449919090438400804119809473510828193277853680977?  
1.70935956599621096961665323217426142432250129115271927421727081345126418270840958764  
0.20928062155561880513383521574600109165595016223940194208811329670902966120239763076  
-0.5640086658743316949169649504841057627079507493269692657938970918611446816147705019  
-3.9163878760412988417823844824224972496552896357084805401330580532711984120662738984  
-3.9163878760412988417823844824224972496552896357084805401330580532711984120662738985  
-0.1896239677148717077867848135314774639427396324956727956498202239926156255505396397  
-8.3314448865464576072681301263403891908158724991609068732210290563657350040610080837  
0.01221270024212726525146175530085564230443557729565259173737937014953607119177084479  
-5.6833861445819475282028086850183211470859225016938029096728255336211073072612356550  
-0.2032957106761212077513652827797140529021521914660693552227252291846608527652939814  
0.01221270024212726525146175530085564230443557729565259173737937014953607119177084479  
0.36760663972523331715484565305606281870030024714465961840220646934618485882418711696  
0.36760663972523331715484565305606281870030024714465961840220646934618485882418711696  
0.91135484231269574356559757648933718558081576164277420003618026206746609779657864122  
-3.5269070873327895209483021827124409351473493815910488005860584027322977173726608987  
1.0000000000000000000000000000000000000000000000000000000000000000000000000000000000  
-2.0992918895414266521279606896868157926869630161666273563493572799874044890908010154  
-0.7219050211235529631148010342234709529448155027649250382675856210297413501282600045  
1.2211346818313407599510039029259833528437758644426009468307074957696062205464810128?  
1.2211346818313407599510039029259833528437758644426009468307074957696062205464810128?  
-0.1782379744530574725397480100122832889049714541539048967910761953484570230560820609  
3.0120227558270822832111535049780248505422425947912817619756640109537928333063672701?  
-0.4738422296447739546165462473367172504777705695941163276972934485792921130035047026  
-0.1675841726931527902791150538452359685135143064856526817170958953458103457900660017  
1.4863873630734431864429137715885416102121244115804981799318971956361879766402711672?  
-0.2694197984117170135379965433432045341490065853633603241886190283736905419231446578  
0.1797261690753711348130963118322821730209412811582170693860257210276686223001141572?  
0.?e-83 + 0.8687580811009225325641138242672332083972288455208809874223601655333152969  
0.?e-83 + 1.1510684294674563826515327418555334611603182386175826826921685831324596077  
-0.6914959378738733968547673102869739976168823998111867521608741386614907210702821410
```

0.04202228714190888728018761901823937129368654024622877130222077502293155331773786720  
-0.4567796350837621444517219691915359374838842206392729151581520491524068154329495287  
0.02529039580593515910796683266021753608516508320911317924180222538905100848224557266  
-5.80941165222275990587928835268479758957368651032573755762232565795686134586854009?  
0.46621545480860202040593114901474448638580844698623307145225365217908762449887087124  
-0.4148361249737683561953407058590472753984567850029017542520863476655684351932416223  
0.56988480121668760429236442736161328148657452102151569199988419640101838120630070348  
0.2531187225327077753184699058888394458338620658682393836707154074816357521262866140  
-4.664941663262068709096473390989584342586028760396197888994177500915502637849068949?  
-0.0139532590782699191544828602485747851091067751731263864565571554016971637890835168  
0.61847530568517107701875567737849207549074921220590410664988434707127887702187371281  
0.1358010443507609500150395927753492148079144203762887988098742955671199504590803204?  
1.5640086658743316949169649504841057627079507493269692657938970918611446816147705019?  
1.20329571067612120775136528277971405290215219146606935522272522918466085276529398148  
-0.7093595659962109696166532321742614243225012911527192742172708134512641827084095877  
-0.0848759938846083672912915840617819982876924433246755706950086302923449247992125678  
1.721905021123552963114801034223470952944815502764925038267585621029741350128260005?  
-0.2345779803307801658538594703538840356540380095458967363805633293792595821034066851  
-1.1444690581489197774198645950663827276444120375699855568332787796909811012969547751  
4.916387876041298841782384482422497249655289635708480540133058053271198412066273899?  
1.721905021123552963114801034223470952944815502764925038267585621029741350128260005?  
-0.1077645942816079961870682930485625270195519445931667401007744452700632399144764563  
-0.221134681831340759951003902925983352843775864442600946830707495769606220546481013?  
1.0616461204303140535980325153267522351539572549564881440362456980856799731381562182?  
0.2057910466220203149492342777814187089071119610322709468523240770182498567254017635?  
-0.4235917619948714834039638007984608749915963542375574893817849221149233397482024639  
0.21816172686375527840851637757969665055060201426723651404564681980162940164737131763  
-0.3823694668070111407867643021108731232342555340758886043375788594237480073077200836  
0.4648852571591930603990729890914121371615404728402263836022303203616426714806742454?  
-0.2733934503542316334836891996375271489939327124519011382500907603116830971457252252  
0.51646848750524897094817152496714627932627604459561527252717631239591538278116286255  
0.07599546705081920438755008143654095134298855098454096235767472542086747837362364249  
1.20329571067612120775136528277971405290215219146606935522272522918466085276529398148  
-0.0848759938846083672912915840617819982876924433246755706950086302923449247992125678  
-0.0508145966661836477655680171668965238512322297698456205386128384330057309835542171  
1.2463382901665493722414387496123370420797260125744516744058196925365030691754092322?  
4.526907087332789520948302182712440935147349381591048800586058402732297717372660899?  
1.2463382901665493722414387496123370420797260125744516744058196925365030691754092322?  
4.526907087332789520948302182712440935147349381591048800586058402732297717372660899?  
1.7614550836896031964394168216217668632474052714283993265440637665262410645798318400?  
0.1306813650432422752153782975907805219730810728166127316540030042201647851765983814?  
-1.7395091509872900175285551909639761438344101678601976900630471186961457625873994341  
0.51646848750524897094817152496714627932627604459561527252717631239591538278116286255  
-3.855090132872401722861657646106789147542595520681030857525699736419595999773514410?  
0.52125597955736976189709317068343991827380383261165481645513810519334600510169714078  
1.6675086881353791732615520162612695529592261805299958632229290515857805276042097554?  
1.14589336788409514780337439881818884872071771066732837473928614369933212196983754050  
-0.0146752385235411136365746080941738098207915982031430245626654052218699661463602453

```
-0.2007573092593308138481650829906194974580976484826870408425751619485722190612951480  
-0.1981169251615481458196746042941686667835657510260119414296711832679352524440710066
```

```
In [18]: len(K.isomorphisms_to(K))
```

```
Out[18]: 2
```

```
In [19]: G=K.symmetry_group()
```

```
In [21]: G.is_amphicheiral()
```

```
Out[21]: True
```
